# Supplementary material for: Climate of the Field: Snowmass 2021
Source: arXiv:2204.03713 source file (2022-09-29)
Supplement: Supplementary file 1 [file AdditionalResources.tex]

\newcommand{\link}[1]{\href{#1}{link}}
% \section{Misc References} 
% \subsubsection{Codes of Conduct}
% \begin{itemize}
% \item Instituto Nazionale di Fisica Nucleare (INFN) (\link{https://home.infn.it/images/cug/Codice_Etico_INFN_EN.pdf})
%     \item NOvA (\link{https://drive.google.com/file/d/14BjLJ6ezCtdXmdlPPTjbYJ28dthA-UsF/view?usp=sharing}), which draws heavily from LSST/DESC (\link{https://lsstdesc.org/assets/pdf/policies/LSST_DESC_Professional_Conduct.pdf})
%     \item nEXO (\link{https://nexo.llnl.gov/diversity-equity-and-inclusion})
%     \item American Physical Society (APS) Meetings (\link{https://www.aps.org/meetings/policies/code-conduct.cfm})
%     \item American Astronomical Society (AAS)  (\link{https://aas.org/policies/ethics})
% \end{itemize}

% \subsubsection{Climate Statements}
% \begin{itemize}
%     \item Wright Laboratory @ Yale (old statement: \link{https://drive.google.com/file/d/17RkY60iNyQICEi2NqOlc-Q1xIApk9Wk0/view?usp=sharing}, now merged with Yale Physics)
%     \item LIGO scientific collaboration (\link{https://dcc.ligo.org/LIGO-M1400285/public})
%     \item American Institute of Physics (AIP) Diversity Statement (\link{https://www.aip.org/diversity-initiatives/diversity-statement})
% \end{itemize}

\subsection*{Diversity and Inclusion Publications / Presentations}
\begin{itemize}
    \item “Diversity Charter of APPEC, ECFA, NuPECC” (\link{http://www.nupecc.org/jenaa/docs/Diversity_Charter_of_APPEC__ECFA__NuPECC-9.pdf})
    \item “Diversity and Inclusion in the CMS Collaboration” (ICHEP 2020) (\link{https://indico.cern.ch/event/868940/contributions/3801003})
    \item “Diversity and Inclusion Activities in the Belle II Collaboration” (ICHEP 2020) (\link{https://indico.cern.ch/event/868940/contributions/3801008/})
    \item "LGBTQ+ Inclusivity in High Energy Physics" (ICHEP 2020) (\link{https://indico.cern.ch/event/868940/contributions/3801005/})
    \item "The Early Career, Gender \& Diversity at LHCb" (ICHEP 2020) (\link{https://indico.cern.ch/event/868940/contributions/3801001/})
    \item "Early Career Initiatives at LHCb" (ICHEP 2020) (\link{https://indico.cern.ch/event/868940/contributions/3801000/})
    \item “Studies related to gender and geographic diversity in the ATLAS Collaboration” (ATL-GEN-PUB-2016-001) (\link{https://cds.cern.ch/record/2202392?ln=en})
    
    \item “An IDEA for Physics Organizations” APS Inclusion, Diversity, and Equity Alliance (APS-IDEA) (\link{https://www.aps.org/programs/innovation/fund/idea-physics.cfm})
    \item “How to Respond to Code of Conduct Reports” (\link{https://files.frameshiftconsulting.com/books/cocguide.pdf})
\end{itemize}

% \subsection{Resources}

\subsection*{Theses}
\begin{itemize}
    \item A Different Kind of Dark Energy: Placing Race and Gender in Physics by Lauren Chambers, Ph.D. (\link{https://laurenmarietta.github.io/pdfs/Chambers_ADifferentKindOfDarkEnergy.pdf})
    \item Gender, Ethnicity, and Physics Education: Understanding How Black Women Build Their Identities as Scientists by Katemari Diogo da Rosa, Ph.D. (\link{https://search.proquest.com/docview/1282654401})
\end{itemize}

\subsection*{Articles}
\begin{itemize}
    \item The 'Benefits' of Black Physics Students by Jedidah C. Isler, Ph.D. (NYT op-ed) (\link{https://www.nytimes.com/2015/12/17/opinion/the-benefits-of-black-physics-students.html})
    \item Disentangling anti-Blackness from physics by Charles D. Brown II, Ph.D. (Physics Today) (\link{https://physicstoday.scitation.org/do/10.1063/PT.6.3.20200720a/full/})
    \item Understanding and Promoting Diversity and Inclusion in Physics (SPS letter from Geraldine Cochran, Ph.D.) (\link{https://www.spsnational.org/the-sps-observer/winter/2017/understanding-and-promoting-diversity-and-inclusion-physics})
    \item The Status of the African-American Physicist in the Department of Energy National Laboratories by Keith H. Jackson, Ph.D. (APS News) (\link{https://www.aps.org/publications/apsnews/200205/backpage.cfm})
\end{itemize}

\subsection*{Funding Resource Documents}
\begin{itemize}
    \item DoE Office of Science: High Energy Physics Advisory Panel (HEPAP), July 2020
    \item Office of Science Diversity, Equity, \& Inclusion Initiatives  (\link{https://science.osti.gov/-/media/hep/hepap/pdf/202007/14-Carruthers-Diversity_Equity_and_Inclusion_in_the_DOE_Office_of_Science.pdf?la=en&hash=C0BF29C74FE960DD64EEC2DB327BEDB09C14816D})
    \item FESAC Report 2020 (\link{https://usfusionandplasmas.org/wp-content/themes/FESAC/FESAC_Report_2020_Powering_the_Future.pdf})
    \item Government-Wide Diversity and Inclusion Strategic Plan 2011 (\link{https://www.opm.gov/policy-data-oversight/diversity-and-inclusion/reports/governmentwidedistrategicplan.pdf})
\end{itemize}

\subsection*{Professional Organizations}
\begin{itemize}
    \item AIP TEAM-UP Full Report (\link{https://www.aip.org/sites/default/files/aipcorp/files/teamup-full-report.pdf})
    \item Inclusive Scientific Meetings Guide (500 Women Scientists) (\link{https://static1.squarespace.com/static/582cce42bebafbfc47a82b04/t/5ca0fe7d9b747a3d7dc7a71f/1554054781756/Formatted+Inclusive+Meeting+Guide-v5.pdf})
    \item LGBT+ Inclusivity in Physics and Astronomy: A Best Practices Guide (\link{https://arxiv.org/pdf/1804.08406.pdf})
    \item NASEM. 2020. The Impacts of Racism and Bias on Black People Pursuing Careers in Science, Engineering, and Medicine: Proceedings of a Workshop. Washington, DC: The National Academies Press. https://doi.org/10.17226/25849. 
    \item NASEM. 2020. Promising Practices for Addressing the Underrepresentation of Women in Science, Engineering, and Medicine: Opening Doors. Washington, DC: The National Academies Press. https://doi.org/10.17226/25585
    % \item Astro Decadal Survey (\link{https://www.nationalacademies.org/our-work/decadal-survey-on-astronomy-and-astrophysics-2020-astro2020}), or more specifically Appendix N (on Equity initiatives) (\link{https://drive.google.com/file/d/1ZyHlBe7wqb-jpFtVBZSVqyNcBQ9Rafuk/view?usp=sharing})
\end{itemize}

% \subsubsection{Public Initiatives}
% \begin{itemize}
%     \item Change-Now Physics: Calls to Action from Black Scientists at Fermilab (\link{https://changenowphysics.com/strategic-plan/})
%     \item \#BlackInAstro stories from astrobites (AAS) (\link{https://astrobites.org/?s=\%23BlackInAstro})
%     \item "How to Respond to Code of Conduct Reports" (\link{https://files.frameshiftconsulting.com/books/cocguide.pdf}) by authors of the Ada Initiative Anti-Harassment framework (\link{https://adainitiative.org/continue-our-work/conference-policies/})

% \end{itemize}
